# Supplementary material for: Learning Graphical Models from a Distributed Stream
Source: arXiv:1710.02103 source file (2017-10-05)
Supplement: Supplementary file 1 [file appendix.tex]

%------------------
\section{APPENDIX}
\label{appendix}
%------------------
\begin{fact}
\label{fact:math-fact}
When $0<x<0.3$, $e^x < 1+2x$ and  $e^{-2x} < 1-x$.
\end{fact}
\begin{proof}
Let $f(x)=e^x-2x-1$, we have 
\[
f'(x)=e^x-2<0 \quad \text{when} \quad 0<x<0.3
\] 
So $f(x)<f(0)=0$, $e^x<1+2x$. 

Similarly, let $g(x)=e^{-2x}-1+x$, 
\[
g'(x)=1-2e^{-2x}<0 \quad \text{when} \quad 0<x<0.3
\]
So $g(x)<g(0)=0$, $e^{-2x}<1-x$.
\end{proof}
%-------------

\begin{lemma}[Lemma~\ref{lem:uniform-approx} restated]
\label{lem:uniform-approx-append}
For $0< \eps <1$ and $n \in \mathbb{Z}^+$, when $\alpha \leq \frac{\eps}{3n}$
\[ \textstyle
\left( \frac{1+\alpha}{1-\alpha} \right)^n \leq e^{\eps} 
\quad and \quad
\left( \frac{1-\alpha}{1+\alpha} \right)^n \geq e^{-\eps}
\]
\end{lemma}
\begin{proof}
When $\alpha \leq \frac{\eps}{3n} \leq \frac{1}{3}$, we have that $\frac{2\alpha}{1-\alpha} \leq 3\alpha$,
\[
\left(\frac{1+\alpha}{1-\alpha}\right)^n  =  \left(1 + \frac{2\alpha}{1-\alpha}\right)^n  
 \leq \left(1 + 3\alpha \right)^n   \leq (e^{3\alpha})^n  \leq e^{\eps}
\]
So $\left( \frac{1+\alpha}{1-\alpha} \right)^n \leq e^{\eps}$ is proved. As
$
\left(\frac{1-\alpha}{1+\alpha}\right)^n = \frac{1}{\left(\frac{1+\alpha}{1-\alpha}\right)^n} \geq e^{-\eps}
$, simultaneously we prove that 
$\left( \frac{1-\alpha}{1+\alpha} \right)^n \geq e^{-\eps}$.
\end{proof}
%------------------------------------------
